# Supplementary material for: Runtime Enforcement of Hyperproperties
Source: arXiv:2203.04146 source file (2022-03-08)
Supplement: Supplementary file 1 [file appendix.tex]

%===========================================
\appendix
%===========================================

\newcommand{\finTinf}{\mathcal P^*(\Sigma^\omega)}

\newpage

\section{Definition: Parity Games}
\label{app:parity}
For a set $A \subseteq I \cupdot O$, $\inputs{A}$ denotes the input-projection on $A$. Analogously, $\inputs{t}$ is the input-projection on a trace $t$ and $\inputs{T}$ the input projection on a set of traces. We use the analogous notation for output projection.

A \emph{parity game} $\game$ is a two-player game defined by a tuple  $(V_0, V_1, \Sigma_0, \Sigma_1, E_0, E_1, v_\mathit{in}, c)$, where $V_0$ and $V_1$ are the states belonging to player $P_0$ and $P_1$, respectively, $\Sigma_0$ and $\Sigma_1$ are the sets of actions, $E_0: V_0 \times \Sigma_0 \rightarrow V_1$ and $E_1: V_1 \times \Sigma_1 \rightarrow V_0$ are the transition functions, $v_\mathit{in} \in V_0$ is the initial state and $c: V_0 \cupdot V_1 \rightarrow \NN$ is the coloring function.
States belonging to $P_0$ and $P_1$ are required to alternate along every path in a Parity game.
For an infinite decision sequence $w = w^0_0 w^1_0 w^0_1 w^1_1 \ldots$, where the two players choose one of their possible actions in every step (i.e., $\forall i \in \NN \ldot w^0_i \in \Sigma_0 \text{ and } w^1_i \in \Sigma_1$), the game generates an infinite play $r = v^0_0 v^1_0 v^0_1 v^1_1 \ldots$, where $v^0_0$ is the initial state and the edge function is followed according to $w$, i.e., $\forall i \in \NN \ldot p \in \set{0, 1} \ldot v^{1-p}_{i+p} = E_p(v^p_i, w^p_i)$. 
The play $r$ is winning for player $P_0$ if and only if the highest color occurring infinitely often in the sequence $c(v^0_0) c(v^1_0) c(v^0_1) c(v^1_1) ...$ is even. 
Otherwise, player $P_1$ wins.
 
A strategy maps the history of the play to the next move that should be executed by the player whose turn it is. 
The strategy for player $P_0$ is a function $\sigma_0: (\Sigma_0 \times \Sigma_1)^* \rightarrow \Sigma_0$, the strategy for player $P_1$ is a function $\sigma_1: (\Sigma_0 \times \Sigma_1)^* \times \Sigma_0 \rightarrow \Sigma_1$. 
A decision sequence $w$ is conforming to a strategy $\sigma_p$ for $p \in \set{0, 1}$, if $\forall i \in \NN$ we have that $w^p_i = \sigma_p(w^0_0 w^1_0 ... w^{1-p}_{i+p-1})$. 
A strategy $\sigma_p$ is called \emph{winning} for player $P_p$ if all decision sequences $w$ conforming to $\sigma_p$ generate plays that are winning for player $P_p$. 
There always exists a winning strategy for exactly one of the players since parity games are \emph{determined}~\cite{MemorylessDetermined}. 
A state $v \in V_0 \cupdot V_1$ is called winning for player $P_p$ if this player has a winning strategy in the modified game $\game^v$ where the initial state $v_\mathit{in}$ is set to $v$. 
The set of all states that are winning for player $P_p$ is called the \emph{winning region} for player $P_p$. 
Parity games are even \emph{memoryless determined}, i.e., if player $P_p$ has a winning strategy in state $v$, then $P_p$ has a \emph{positional strategy} $\sigma: V_p \rightarrow \Sigma_{p}$, such that for any decision sequence conforming to $\sigma$, the play starting in $v$ is winning for $p$. Positional strategies give a decision for each of the player's states, independently of the history of the play. The exact complexity of parity game solving, i.e. determining the winning regions, is still unknown. Current state-of-the-art algorithms perform in quasi-polynomial time~\cite{DBLP:conf/mfcs/Parys19}.

\subsection{Parity Games vs Synthesis}

There is a strong correspondence between parity games and reactive synthesis.
Strategies for parity games induce implementations (i.e., strategy functions) for reactive systems. 
Player $P_0$ represents the system and controls the outputs, and player $P_1$ represents the environment controlling the inputs. 
Given a parity game $\game$ and a word $u_1 \ldots u_i \in (\pow{I \cupdot O})^*$, the word corresponds to a decision sequence $u_{1|O} u_{1|I} \ldots u_{i|O} u_{i|I}$ and a corresponding run $v^0_0 v^1_0 \ldots v^0_i v^1_i$ with $v^0_0 = v_\mathit{in}$ in  $\game$.
Let a strategy $\sigma_0$ for the system player $P_0$ in a parity game $\game$ with action sets $\Sigma_0 = 2^O, \Sigma_1 = 2^I$ be given. For a sequence $w = w_0^1 \ldots w_i^1 \in (\pow{I})^*$, let $d_w = w_0^0 w_0^1 \ldots w_{i}^0 w_{i}^1$ be the corresponding decision sequence conforming to $\sigma_0$. We define $\sigma : \strat{I}{O}$  for $w = w_0 \ldots w_i \in (\pow{I})^*$ as $\sigma(w) = \sigma_0(d_w)$.
A given LTL formula $\varphi$ can be translated to a parity game $\game_\varphi$ via deterministic parity automata in doubly-exponential complexity~\cite{DBLP:conf/tacas/EsparzaKRS17}. 
Formula $\varphi$ is realizable iff the game $\game_\varphi$ is won by player $P_0$. 
Its winning strategy~$\sigma_0$ induces the reactive strategy $\sigma$ representing a system implementation that satisfies~$\varphi$. 

\begin{example}
	Fig.~\ref{fig:ParityGame} depicts a parity game for observational determinism as described in Section~\ref{sec:requirements_models}. Let $\Sigma_{0} = \set{o_1, o_2}$ be the set of low-security outputs and $\Sigma_{1} = \set{i_1, i_2}$ be the set of low-security inputs. As long as $i_1$ and $i_2$ agree, $o_1$ and $o_2$ also have to agree. In this simplified example, a winning strategy would be to always choose $o_1$ equivalent to $o_2$, independently of the inputs.
	
	\begin{figure}[t]
		\centering
		\begin{tikzpicture}[->,>=stealth',shorten >=1pt,auto,node distance=1.3cm,semithick]
		\tikzstyle{every state}=[draw, align=center]
		\tikzstyle{every text node part}=[align=center,font=\scriptsize]
		
		\node[initial,state]   (I)                  at (-1,0) {$q_0$ \\ $0$};
		\node[state,rectangle, minimum width={1.5cm}] (IE) at (2.5,0)     {$q_0, \emptyset$ \\ $0$};
		\node[state,rectangle, minimum width={1.5cm}] (IO) [above of=IE]    {$q_0, \set{o_1, o_2}$ \\ $0$};
		\node[state,rectangle, minimum width={1.5cm}] (I1) [below of=IE]    {$q_0, \set{o_1}$ \\ $0$};
		\node[state,rectangle, minimum width={1.5cm}] (I2) [below of=I1]    {$q_0, \set{o_2}$ \\ $0$};  
		\node [state] (A) at (5.5,0) {$q_\top$ \\ $0$};
		\node [state,rectangle] (AE) at (7,0) {$q_\top, \_$ \\ $0$};
		\node (helper) [below of=A] {};
		\node (helperE) [below of=AE] {};
		\node[state] (R) [below of=helper] {$q_\bot$\\ $1$ };
		\node[state,rectangle] (RE) [below of=helperE] {$q_\bot, \_$\\ $0$ };
		
		\path (I.70)  edge [line width=1.3pt,bend left]  node [above left] {$\set{o_1, o_2}$} (IO.160)
		(I.325) edge [line width=1.3pt,bend right] node [below]      {$\emptyset$}      (IE.205)
		(I.300) edge [bend right] node [below]      {$\set{o_1}$}      (I1.180)
		(I.270) edge [bend right] node [below left] {$\set{o_2}$} (I2.180)
		
		(IO.205) edge node [above] {$\set{i_1, i_2}$ $\lor \emptyset$} (I.30)
		(IO.23) edge node [above right] {$\set{i_1} \lor \set{i_2}$} (A.110)
		
		(IE.175) edge node [below] {$\set{i_1, i_2} \lor \emptyset$} (I.10)
		(IE.5)  edge node {$\set{i_1} \lor \set{i_2}$} (A.170)
		
		(I1.360) edge node [above] {$\set{i_1} \lor \set{i_2}$ \phantom{mm}} (A.210)
		(I1) edge node {$\set{i_1, i_2} \lor \emptyset$} (R)
		
		(I2.20) edge node [above right] {\phantom{m} $\set{i_1} \lor \set{i_2}$}      (A.250)
		(I2)    edge node [below] {$\set{i_1, i_2} \lor \emptyset$} (R)
		
		(A)  edge [line width=1.3pt,bend right] node {$\top$} (AE)
		(AE)  edge [bend right] node [above] {$\top$} (A)
		(R)  edge [bend right] node {$\top$} (RE)
		(RE)  edge [bend right] node [above] {$\top$} (R)
		;
		
		\draw[dotted,-] (-1.3,-0.7) -- (7,-0.7);
		\node (win) at (-2,-0.5) {\textit{winning}};
		\node (los) at (-2,-0.9)  {\textit{losing}}; 
		\end{tikzpicture}
		\caption{Parity game for observational determinism. States of the system player $P_0$ are depicted as circles. $P_0$ has a winning strategy from the upper states using only bold transitions from system states. }
		\label{fig:ParityGame}
		\vspace{-10pt}
	\end{figure}
\end{example}

\section{Parallel Model, Non-Reactive Enforcement}

In general, we assume systems to be reactive. There are however situations in which the enforcer does not need to distinguish between inputs and outputs. This is the case, for example, when monitoring the outgoing stream of a device to a cloud like in the fitness-tracker example given in the introduction. We show that in such a situation, it is not necessary to build a parity game. Indeed, existing algorithms for HyperLTL monitoring~\cite{monitoring_hyperproperties_journal} can be easily extended to also enforce a hyperproperty. 
In~\cite{monitoring_hyperproperties_journal}, monitoring of HyperLTL formulas is studied with respect to both trace input models. Their algorithm for the parallel model already recognizes minimal bad prefixes. We can therefore concentrate on how to provide a valid continuation once a minimal bad prefix is detected.
%We give an algorithm for HyperLTL formulas interpreted with the infinite semantics. 
%The solution can be generalized to the finite trace semantics.
%The finite semantics can be easily encoded in the infinite semantics by adding a proposition $\mathit{end}$ denoting the end of the trace (see Appendix~\ref{ap:finite}).

Let a HyperLTL formula $\varphi$ from the universal HyperLTL fragment, and the number of traces $n$ be given. Assume that a HyperLTL monitor for the parallel trace input model is running.
%Assume we want to enforce a system that produces $b$ traces in parallel. 
Each event $e^i$ consists of a tuple $(e_1^i, \ldots , e_n^i) \in (2^{\Sigma})^n$. 
%We store the sequence of events $e^1, \ldots , e^i$ observed so far. 
As long as the monitor does not raise an alarm, new events are forwarded to the monitor.
%If the monitor does not raise an alarm, the enforcer indicates that it has accepted $e^i$. 
If the monitor raises an alarm at position $i+1$, we encode the observed traces up to position~$i$ into a HyperLTL formula, together with the formula we want to enforce. 
The resulting formula is the following.
\begin{alignat}{2}
\psi \coloneqq ~ & \exists \pi_1 \ldot \ldots \exists \pi_n \ldot \varphi ~ \land \label{form:orig}\\
&\bigwedge_{1 \leq k \leq n} ~ \bigwedge_{0 \leq j \leq i} \X ^{j} (\bigwedge_{a \in e_k^j} a_{\pi_k} \land  \bigwedge_{a \notin e_k^j} \neg a_{\pi_k}) \label{form:b_traces} 
\end{alignat}
We use $\X ^j$ as an abbreviation for $j$ consecutive $\X$.
Formula~\ref{form:orig} ($\varphi$) is the original universal HyperLTL formula.
Formula~\ref{form:b_traces} ensures that a satisfying trace set contains at least $n$ traces with the prefixes seen so far. 
The resulting formula $\psi$ is an $\exists^*\forall^*$ HyperLTL formula. 
It is forwarded to the SAT solver which, if the result is SAT, returns at least $n$ traces $(t_1, \ldots , t_n)$ such that the traces $(t_1[i+1 \ldots], \ldots , t_n[i+1 \ldots])$ can be used to continue the observed prefix and enforce $\varphi$.
%such that the trace set $\set{e_j^0 \ldots e_j^{i} ~ t_j[0 \ldots] ~|~ 1 \leq j \leq n}$ fulfills $\varphi$. 
Note that we did not ask for \emph{exactly} $n$ traces. 
Universally quantified HyperLTL formulas are downwards closed, i.e., any additional traces returned by the SAT solver can just be ignored.
Also note that the result must be SAT by construction. If the result was UNSAT, then the already observed prefix up to position $i$ would form a minimal bad prefix. Then, the monitor would have raised an alarm at position $i$ already.

Compared to the parity-game-based algorithms for reactive systems, we do not solve a synthesis problem, but a satisfiability problem. Satisfiability of $\exists^*\forall^*$ HyperLTL formulas is solvable in single-exponential space, compared to the triple exponential time complexity for the reactive case. However, the parity game can be computed beforehand, while the satisfiability problem needs to be solved at runtime (since we need to encode the observed traces). The evaluation of these two approaches thus depends on the specific situation at hand, i.e., on whether the parity game can be computed at all and what computational overhead at runtime is considered acceptable. 

This algorithm takes over the control of the enforced system when a bad prefix was about to occur. 
The enforcer then fully determines how the system executions are continued in the future. 
If we only want to avoid the violation of the specification in the current situation but give back the control to the system afterwards, this algorithm can be adapted accordingly: 
Given a monitor alarm at position $i+1$, we solve the above formula $\psi$ and use $(t_1[i+1], \ldots, t_n[i+1])$ as the event for position $i+1$. 
After that, we go back to monitoring the system for the next bad prefix. In order to give a correct enforcement, even only for one position, one still has to compute a solution for all coming positions. Otherwise, there might be no valid continuation in the future.

\section{Sequential Model}
\label{app:bounded_sequential}

\subsection{Distributed Architectures}

A \emph{distributed architecture}~\cite{conf/focs/PnueliR90,conf/lics/FinkbeinerS05} $\mathcal{A}$ over $\Sigma$ is a tuple $\langle P,p_\mathit{env},\mathcal{I},\mathcal{O} \rangle$. $P$ is a finite set of processes and $p_\mathit{env} \in P$ is the designated environment process. Furthermore, functions $\mathcal{I}: P \rightarrow 2^\Sigma$ and $\mathcal{O}: P \rightarrow 2^\Sigma$ indicate inputs and outputs of processes. The output of the processes must be pairwise disjoint, i.e., for all $p \ne p' \in P$ it holds that $\mathcal{O}(p) \cap \mathcal{O}(p') = \emptyset$. Additionally, we assume that $\mathcal{I}(p_\mathit{env}) = \emptyset$.
An LTL formula $\varphi$ over $\Sigma$ is \emph{realizable} in an architecture $\langle P,p_\mathit{env},\mathcal{I},\mathcal{O} \rangle $ if for each process $p \in P$, there is a strategy $\sigma_p \colon \strat{\mathcal{I}(p)}{\mathcal{O}(p)}$ such that all $\sigma_p$ toghether satisfy $\varphi$.
The synthesis of distributed architectures from an LTL specification is decidable if the processes in the architecture can be ordered linearly according to their ``level of informedness". Formally, we define the informedness relation $\leq$ on processes $p$ and $p'$ as $p \leq p'$ iff $\mathcal{I}(p) \subseteq \mathcal{I}(p')$. If the informedness relation in the set of processes is a linear preorder, $\mathcal{A}$ is called \emph{hierarchical}. As an example for a (hierarchical) distributed architecture, consider Figure~\ref{fig:archs}.
\begin{figure}[t]
	\centering
	\begin{tikzpicture}[->,>=stealth',shorten >=1pt,auto,semithick,scale=1,transform shape,scale=0.8]
	\tikzstyle{every state}=[shape=rectangle]
	\tikzstyle{envstate}=[shape=circle,scale=0.9]	
	\node [state,envstate] (e) {$env$};
	\node [state, below left=0.8 of e] (a) {$p_0$};	
	\node [state, below right=0.8 of e] (b) {$p_b$};
	\node [below = 0.5 of e, xshift=-3ex] (c) {};		
	\node [below = 0.5 of e, xshift=3ex] (d) {};			
	\path (a) -- (b) node[midway, below=0.1 of e] (dots) {$\cdots$};
	\path[->]
	(e) edge (c)
	(e) edge (d)
	(e) edge node [label,above left = 0 and -0.1] {$I_1$} (a)
	(e) edge node [label,above right = 0 and -0.1] {$I_b$} (b)
	(a) edge node [label,above left = -0.15 and 0] {$O_1$} +(0,-1.3)
	(b) edge node [label,above right = -0.15 and 0] {$O_b$} +(0,-1.3)
	;
	\end{tikzpicture}
	\caption{Distributed architecture $\mathcal{A}$, which is hierarchical if $I_1 \subseteq \ldots \subseteq I_b$.}
	\label{fig:archs}
\end{figure}
\subsection{Proof of Theorem~\ref{thm:Bounded_Sequential_Pipelines}}
For a formal proof of the sketched reduction, we need to introduce the notion of past-only strategies in the sequential model.
A strategy in the sequential model is a past-only strategy, if it does not depend on the inputs of already observed sessions that lie in the future compared to the current session. Formally:
\begin{definition}[Past-only Strategy for Sequential Model]
	Let $\sigma$ be a hyper-prefixed stategy. $\sigma$ is \textit{past-only}, if for any $i \in \mathbb{N},~ U_1, U_2 \in \finTinf$ with $U_1[0,i] = U_2[0,i]$ and $U_{1|O}[i, \infty] = U_{2|O}[i,\infty]$ and $u \in (\pow{I})^*$ with $|u| = i$, it holds that $\sigma(U_1)(u) = \sigma(U_2)(u)$.
\end{definition}
In the above definition $U_{|O}$ denotes the projection of $U$ on its outputs.
In the following, strategy are always considered to be strategies in the sequential model.

\begin{lemma}
	Given an enforceable universal HyperLTL formula $\varphi$, a prefix $(U,u)$ is losing for $\varphi$ with past-only strategies iff it is losing for $\varphi$ with normal hyper-prefixed strategies.
\end{lemma}
\begin{proof}	
	Let $\varphi$ be a universal HyperLTL formula. If some $(U,u)$ is losing with normal strategies, it is clearly also losing with past-only strategies. For the other direction, assume that $(U,u)$ is winning with a normal strategy $\sigma$, but losing for all past-only strategies. Then, $\varphi$ must relate an output $o$ at position $i = |u|$ with an input from a trace from $U$ at a position $j > i$. Since $(U,u)$ is losing for all past-only strategies, for any choice for $\sigma(U)(u)$, there is a $u' \in U$, such that iff $u'[j]$ was chosen differently, $\sigma(U)(u)$ would change.
	This implies that $\varphi$ is not enforceable: Consider the case where $U = \emptyset$. Let $\sigma(\emptyset)(u) = o$ be the output obtained by the strategy. At position $j$, the environment chooses an input which would have led to a change of $\sigma(U)(u)$ for the case that $\sigma(U)(u) = o$ as described above. Therefore, $\varphi$ evaluates to false on the resulting trace set (with a single trace), since $\varphi$ is a univeral property.
%	Let $U'$ be a set of traces with $U[0,i] = U'[0,i]$ and $U_{|O}[i, \infty] = U^\prime_{|O}[i,\infty]$ such that $\sigma(U)(u) \neq \sigma(U')(u)$. Such a $U'$ exists, because otherwise, $(U,u)$ would not be losing for past-only strategies. Even more, choosing $\sigma(U')(u)$ in the place of $\sigma(U)(u)$ would be losing for $\sigma$.
%	Let $u' \in (\pow{I})^*$ be an input sequence which is a prefix of a trace in $U'$ but not in $U$.
%	We show that $\varphi$ is not enforceable. Consider the case where $U = \emptyset$. Let $\sigma(\emptyset)(u)$ be the output obtained by the strategy. If $\sigma(\emptyset)(u) = \sigma(U)(u)$, then the environment chooses $u'$ as input sequence in the next session. 
\end{proof}
We conclude that $\varphi$ is enforceable in the bounded sequential model iff it is enforceable by a past-only strategy. We continue to prove Theorem~\ref{thm:Bounded_Sequential_Pipelines}.

Recall Theorem~\ref{thm:Bounded_Sequential_Pipelines}: \textit{HyperLTL enforcement in the bounded sequential model can be reduced to the LTL synthesis problem of hierarchical distributed architectures.}

\begin{proof}[Theorem~\ref{thm:Bounded_Sequential_Pipelines}.]
	Let a HyperLTL formula $\varphi$ and a bound $b$ be given. The problem is to detect losing prefixes in the bounded sequential model. Furthermore, for a prefix which is not losing, we need to provide a winning strategy. We first translate the problem into an LTL synthesis problem with an additional requirement on the strategy and then reduce it to LTL synthesis of hierarchical distributed architectures.
	
	We transform the HyperLTL formula $\varphi$ over $\Sigma$ into the LTL formula $\varphi^b_\text{LTL}$ as described in Section~\ref{sec:parallel-algorithms}.
	However, compared to the parallel model, we cannot explicitly spell out the trace relations in LTL.
%	If a new event comes in on trace $t_i$, it is encoded as an additional conjunct into the LTL formula.
%	However, by spelling out the trace relations of the HyperLTL formula in LTL, we do not correctly capture the bounded sequential model.
	A strategy satisfying $\varphi^b_\text{LTL}$ would set the events for all traces at some position $k$ at the same time, but events come in sequentially trace by trace.
	Solving the normal realizability problem for $\varphi^b_\text{LTL}$ would therefore not provide a valid solution.
	To bridge this gap, we add an additional requirement to the strategy: The output for the encoded trace $i$ is not allowed to depend on the inputs for traces $j > i$. To formalize the requirement, let $\Sigma = I \cup O$ with $I$ the inputs and $O$ the outputs. Let furthermore $I_m$ and $O_m$ for $1 \leq m \leq b$ denote the set of annotated inputs and outputs encoding trace $m$. The requirement is the following:
	\begin{alignat*}{2}
	& \text{If } && \sigma(\set{I_1^0 \cup {\ldots} \cup I_i^0 \cup I_{i+1}^0 \cup {\ldots} \cup I_b^0} {\ldots} \set{I_1^k {\ldots} \cup I_i^k \cup I_{i+1}^k \cup {\ldots} \cup I_b^k})\\
	& && = \set{O_1 \cup {\ldots} \cup O_i \cup O_{i+1} \cup {\ldots}\cup O_b}, \\
	& \text{then } && \sigma(\set{I_1^0 \cup {\ldots} \cup I_i^0 \cup \hat I_{i+1}^{0} \cup {\ldots} \cup \hat I_b^{0}} {\ldots} \set{I_1^0 \cup {\ldots} \cup I_i^k \cup \hat I_{i+1}^k \cup {\ldots} \cup \hat I_b^k})\\
	& && = \set{O_1 \cup {\ldots} \cup O_i \cup \hat O_{i+1} \cup {\ldots}\cup \hat O_b}, \\
	\end{alignat*}
	for any $1 \leq i \leq b$, trace position $k$, and for any choice of inputs $I_m^l, \hat I_m^{l} \subseteq I_m$ with $1 \leq m \leq b$ and $1 \leq l \leq k$.
	The equation states that if the strategy is called with a sequence of $k$ events and the inputs encoding the last $b-i$ traces change, then only the outputs encoding the last $b-i$ traces are allowed to change.
	Like this, we require the strategy choice for output for trace $i$ to be independent of all possible inputs for the future traces. 
%	If the strategy now needs to react to an incoming event on trace $i$, then the inputs not known yet can be chosen arbitrarily to get an output from the strategy. 
	With this additional requirement, the LTL realizability problem is equivalent to the HyperLTL enforcement problem in the bounded sequential setting (with past-only strategies). 
	The restriction on the strategy, however, encodes a hierarchical architecture. 
	The strategy for the first trace is ``the least informed", the outputs are only allowed to depend on the inputs for the first trace. 
	The outputs of the second trace are allowed to depend on the inputs of the first two traces, and so on. 
	Finally, the last trace is the most informed. 
	We can thus reduce the problem of finding a strategy with the additional requirement on the strategy to finding strategies for each process in the hierarchical architecture $\mathcal{A}$ depicted in Figure~\ref{fig:archs}. 
	Inputs $I_i$ are the inputs visible to trace $i$, i.e the set $\set{a_j ~|~ a \in I, j \leq i}$ (and analogously for the outputs). The LTL formula remains the same.
	
	Now, the enforcement algorithm for the HyperLTL formula is the following. Before the first event occurs, check if $\varphi^b_\text{LTL}$ is realizable in architecture $\mathcal{A}$. If not, return an error. If an event occurs, it is encoded into the LTL formula with an additional conjunct (c.f. Section~\ref{sec:parallel-algorithms}, the \textit{Monitor} paragraph).
	Check if the formula is still realizable in $\mathcal{A}$. If yes, continue. If not, raise an alarm. If an alarm occurs on trace $t_i$, the prefix up to the alarm was realizable, i.e., there exist strategies for the processes in $\mathcal{A}$. Use strategy $\sigma_i$ to finish trace $t_i$. For future traces $t_j$ with $i < j \leq b$, use strategy $\sigma_j$. 
\end{proof}

The above complexity is strict: It is easy to see that the above reduction can be transformed to reduce the synthesis of hierarchical distributed architectures to enforceability in the bounded sequential model.

\subsection{Non-Reactive Enforcement}
\label{app:sat-2}
Similarly to the parallel input model, we can encode enforcement in the sequential model as a HyperLTL SAT problem, for the special case where the enforcer does not need to distinguish between inputs and outputs. Again, we employ existing monitoring tools and show how to provide an enforcement in case an error is observed.
Let a HyperLTL monitor for the sequential model be given, e.g., the one from~\cite{monitoring_hyperproperties_journal}. 
Note that in the sequential setting, finished sessions naturally produce finite-length traces. We assume that the resulting traces are extended to inifinite ones by appending the trace $\set{\mathit{end}}^\omega$.
Assume a violation of the property is detected in session $n$ at position $c+1$. Furthermore, for each finished session $k < n$, let the trace length be $i_k$.

We remove the last step that caused the violation (since the monitor monitors for minimal prefixes) and solve the satisfiability problem of the following formula
\begin{alignat}{2}
\psi \coloneqq & ~ \exists \pi_1 \ldot \ldots \exists \pi_{n} \ldot && \bigwedge_{1 \leq k < n} \X^{i_k} \Gl \mathit{end}_{\pi_k} \land \bigwedge_{0 \leq j \leq i_k} \X ^{j} (\bigwedge_{a \in e_k^j} a_{\pi_k} \land  \bigwedge_{a \notin e_k^j} \neg a_{\pi_k}) \label{form:b_traces2} \\
& && \bigwedge_{0 \leq j < c} \X ^{j} (\bigwedge_{a \in e_n^j} a_{\pi_n} \land  \bigwedge_{a \notin e_n^j} \neg a_{\pi_n}) \label{form:current_trace} 
\end{alignat}
The first conjunct (Formula~\ref{form:b_traces2}) encodes all finished sessions. 
Formula~\ref{form:current_trace} encodes all events seen so far for the current session $n$.
Any trace set satisfying $\psi \land \varphi$ provides a valid continuation for trace $n$, finishing the current session. Furthermore, for future traces, the enforcer can choose any trace from that trace set (since the specification is universal and the enforcer has control over all atomic propositions).
